# Supplementary material for: OSM-tree: A Sortedness-Aware Index
Source: arXiv:2202.04185 source file (2022-02-08)
Supplement: Supplementary file 1 [file appendix.tex]

\section{Appendix}
\Paragraph{Point Query Modelling} To model the relationship between 
the size of the \pinBufName{} and its overhead on the lookup cost, 
let us assume that the \pinBufName{} size is $S$ and that we have $L$ levels in the 
tree. In order to guarantee that the overhead 
for an existing point query is less than $\delta$ of the standard query, we want the number 
of I/Os in the worse case to be less than $(1+\delta) \cdot \text{query\_cost}$. Here, 
$\text{query\_cost}$ is the standard point query cost in the underlying tree data structure, which 
in our case is either the \bplustree{} or the \bepsilontree{}. We assume that 
a fraction of the OSM Buffer is always unsorted, on average 50\%. For this unsorted part, 
a query will access each partition if the data exists there or if there is a false positive. 
We express the size of the buffer as a fraction of the total data size, $p$, which also means 
that $S=p\cdot N_B$. The probability that a query finds the desired key in the 
unsorted part of the buffer is $50\% \cdot p$, and in the sorted of the buffer it is also 
$50\% \cdot p$, and in the remaining part of the tree the cost is $1-p$. To scan the sorted part, we use a faster 
interpolation search ~\cite{VanSandt2019} that has an $O(log(log(N)))$ cost. 
Thus, on a high level, the total cost of a point 
query on the \sysName{} is: 

\begin{eqnarray}
	0.5\cdot p \cdot \text{search unsorted zones} + 
	\nonumber\\ 0.5\cdot p \cdot\text{search unsorted+sorted zones} + 
	\nonumber\\ (1-p)\cdot \text{search unsorted+sorted zones+tree search} 
	\label{eq:hl_pq_cost_text}
\end{eqnarray}

To optimize query performance, \sysName{} utilizes several layers of zonemaps to filter qualifying keys.
Let $q_o$ be the probability not skipping the \pinBufName{} during a point lookup. Similarly, 
$q_u$ and $q_s$ are probability of not skipping the unsorted section and sorted section of \pinBufName{} 
respectively. Note, when the range of keys in \pinBufName{} and that of the tree overlap, 
$q_o=0$. Eq. ~\eqref{eq:hl_pq_cost_text} can be modified as follows:

\begin{eqnarray}
	0.5\cdot p \cdot \text{search unsorted zones} + \nonumber\\ 
	0.5\cdot p \cdot (q_u \cdot \text{search unsorted}+ \nonumber\\ 
	\text{sorted zones}) + \nonumber\\
	(1-p)\cdot (q_o \cdot \left(q_u \cdot \text{search unsorted}+ q_s \cdot \text{sorted zones}\right) + \nonumber\\
	+\text{tree search})
	\label{eq:basic_pq_cost_text}
\end{eqnarray}

The number of elements that we will be scanning on average in both the sorted and unsorted part of the \pinBufName{}
is equivalent to $\frac{S}{2}$. Let the number of pages filtered by the zonemap in the unsorted section be denoted by the 
zonemap ratio $Z_R$, and the ratio of existing to empty queries be $v$. Assuming the false positive for the global BF is $f_G$ and that 
of each sub-level BF within every zone is $f_p$, we can substitute these 
values in ~\eqref{eq:basic_pq_cost_text}, so the point query cost becomes the following.

\begin{eqnarray}
	0.5\cdot p \cdot \left(v+f_G \cdot Z_R \cdot f_p \cdot \frac{S}{2}\right) + \nonumber\\
	0.5\cdot p \cdot \left(q_u \cdot f_G \cdot Z_R \cdot f_p \cdot \frac{S}{2}+ log_2\left(log_2\left(\frac{S}{2}\right)\right)\right) + \nonumber\\
	(1-p)\cdot \left( q_o \cdot \left(q_u \cdot f_G \cdot Z_R \cdot f_p \cdot \frac{S}{2}+ q_s \cdot log_2\left(log_2\left(\frac{S}{2}\right)\right)\right)\right) + \nonumber\\
	(1-p) \cdot log_B\left(N_B - S\right)\nonumber
	% \label{eq:query_cost_substituted_basic}
	% f_G \cdot Z_R \cdot f_p \cdot \frac{S}{2} + 0.5\cdot p + 
	% (1-0.5\cdot p) \cdot log_2\left(log_2\left(\frac{S}{2}\right)\right)+ \nonumber\\
	% (1-p)\cdot log_B\left(N_B - S\right))=\nonumber\\
	% f_G \cdot Z_R \cdot f_p \cdot \frac{S}{2} + 0.5\cdot \frac{S}{N_B} + 
	% \left(1-\frac{S}{2\cdot N_B}\right) \cdot log_2\left(log_2\left(\frac{S}{2}\right)\right)+ \nonumber\\
	% \left(1-\frac{S}{N_B}\right)\cdot log_B\left(N_B-S\right)\nonumber
\end{eqnarray}

We assume $log_2\left(log_2\left(\frac{S}{2}\right)\right) \approx 1$ 
and $log_B\left(N_B - S\right) \approx log_B\left(N_B\right)$, and substitute $S = p \cdot N_B$ 
to simplify and bound the cost to within 
$(1+\delta) \cdot log_B(N_B)$
as follows. 
\begin{small}{
	\begin{eqnarray}
	% 0.5 \cdot p \cdot \left(v+f_G \cdot Z_R \cdot f_p \cdot \frac{p\cdot N_B}{2}\right) + \nonumber\\
	% 0.5\cdot p \cdot \left(q_u \cdot f_G \cdot Z_R \cdot f_p \cdot \frac{p\cdot N_B}{2}+ 1\right) + \nonumber\\
	% (1-p)\cdot \left( q_o \cdot \left(q_u \cdot f_G \cdot Z_R \cdot f_p \cdot \frac{p\cdot N_B}{2}+ q_s \right)\right) + \nonumber\\
	% (1-p) \cdot log_B\left(N_B\right) = \nonumber \\
	p^2 \cdot \left( f_G \cdot Z_R \cdot f_p \cdot \frac{N_B}{2} \cdot \left( 0.5 + 0.5 \cdot q_u - q_u \cdot q_o \right) \right) + \nonumber\\
	p \cdot \left( 0.5\cdot(v+1) + q_u \cdot q_o \cdot f_G \cdot Z_R \cdot f_p \cdot \frac{N_B}{2} - q_o \cdot q_s - log_B(N_B) \right) + \nonumber\\
	q_o \cdot q_s + log_B(N_B) < (1+\delta) \cdot log_B(N_B) \nonumber
\end{eqnarray}
}\end{small}

% We now want to bound this quantity to within $(1+\delta) \cdot log_B(N_B)$, 
% i.e. within $\delta$ of the standard query cost in \bplustree{}:
% \begin{eqnarray}
% 	p^2 \cdot \left( f_G \cdot Z_R \cdot f_p \cdot \frac{N_B}{2} \cdot \left( 0.5 + 0.5 \cdot q_u - q_u \cdot q_o \right) \right) + \nonumber\\
% 	p \cdot \left( 0.5\cdot(v+1) + q_u \cdot q_o \cdot f_G \cdot Z_R \cdot f_p \cdot \frac{N_B}{2} - q_o \cdot q_s - log_B(N_B) \right) + \nonumber\\
% 	q_o \cdot q_s + log_B(N_B) < (1+\delta) \cdot log_B(N_B) \nonumber
% \end{eqnarray}

At the worst-case, we go into every component of the \sysName{} without skipping, i.e. 
$q_u = q_s = q_o = 1 = Z_R$. Then, our query cost simplifies to a linear term in $p$ and can be 
bound as shown below.
\begin{eqnarray}
	p \cdot \left( 0.5(v+1) + f_G \cdot Z_R \cdot f_p \cdot \frac{N_B}{2} - 1 - log_B(N_B) \right) + \nonumber\\
	1 + log_B(N_B)
		< (1+\delta) \cdot log_B(N_B) \nonumber \\
	% \Rightarrow p \cdot \left( 0.5 \cdot v  + f_G \cdot Z_R \cdot f_p \cdot \frac{N_B}{2} - 0.5 - log_B(N_B) \right) \nonumber\\
	% 	< \delta \cdot log_B(N_B) - 1 \nonumber\\
	\Rightarrow p < 2 \cdot \frac{\delta \cdot log_B(N_B) - 1}{v + f_G \cdot f_p \cdot N_B - 1 - 2log_B(N_B)}
	\label{eq:buffer_size_bound}
\end{eqnarray}

We now try to lower bound the value of $\delta$ for the worst-case scenario, i.e. what is the minimum 
penalty in query cost that we might incur with the \sysName{}. Since $N_B$ is usually large, 
we know that the denominator for the expression in Eq. ~\eqref{eq:buffer_size_bound} will always be positive. 
For eq. ~\eqref{eq:buffer_size_bound} to hold, we need: 
\begin{eqnarray}
	\delta \cdot log_B(N_B) - 1 > 0 
	\Rightarrow \delta > \frac{1}{log_B(N_B)} = \frac{1}{L}
	\label{eq:delta_bound_worst_case}
\end{eqnarray}

% \begin{figure}[t!]
% 	\centering
%     \includegraphics[scale=0.48]{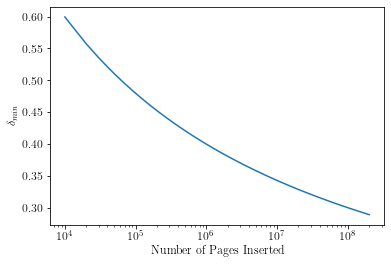}
% 	\caption{The minimum penalty reduces as we insert more pages to the index.}
% \label{fig:deltavnb}
% \vspace{-4mm}
% \end{figure}
% \begin{figure}[t!]
% 	\centering
%     \includegraphics[scale=0.48]{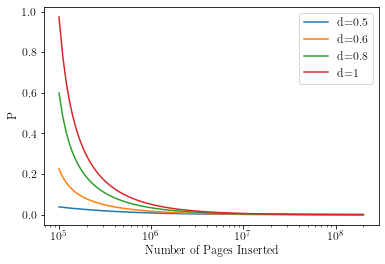}
% 	\caption{As we decrease the penalty ($\delta$), the size of the buffer is limited to 
% 	smaller fraction of the total data size.}
% \label{fig:pvnb}
% \vspace{-4mm}
% \end{figure}

\begin{figure}[!hbt]
    \centering
    \begin{subfigure}[b]{0.23\textwidth}
        \centering
    \includegraphics[scale=0.3]{images/deltavnb.png}
	\caption{Adding more pages to the index reduces the minimum penalty.}
\label{fig:deltavnb}
	\end{subfigure}
	\hfill
    \begin{subfigure}[b]{0.23\textwidth}
        \centering
		\includegraphics[scale=0.3]{images/pvnb.png}
	\caption{Decreasing the penalty ($\delta$) will result in smaller permissable buffer sizes.}
	\label{fig:pvnb}
    \end{subfigure}
\caption{Cost Model Trends}
\label{fig:costmodeltrends}
% \vspace{-4mm}
\end{figure}

Figure ~\ref{fig:costmodeltrends} shows a modelling of how the query cost penalty ($\delta$) and  
size of the buffer ($p$) vary with number of pages inserted into the index. For both trends, we use the 
worst case models for from equation ~\eqref{eq:buffer_size_bound} and ~\eqref{eq:delta_bound_worst_case}, with 
$f_G = f_p = 0.008$, and assume all existing queries ($v=1)$.
 
\subsection{Adaptive Buffer}
In the \sysName{}, we use multiple layers of bloom filters and zonemaps to alleviate the sequential scan cost in the unsorted 
section of the \pinBufName{}. Figure \ref{} shows that the number of pages sequentially scanned is reduced through the filtration 
process. Nonetheless, we still may be required to scan at most $50\%$ of the buffer, which still is expensive. To reduce this overhead, 
we explore the adaptability of the \pinBufName{}. Interpolation scan definitely amortizes the query cost, but it cannot be used in the 
unsorted section due to its requirement of sorted order. To this end, we initate a sorting step during point lookups that 
would establish complete order in a part of the unsorted section. We also introduce a threshold that defines the criteria for sorting.  
In case of continuous queries, we conjecture that absorbing a sorting cost in one query will benefit all lookups that follow. 

Suppose after a flush cycle, $50\%$ of the buffer is sorted. We then have a few inserts that fill up $o$ pages 
of the buffer $\left(o < \frac{S}{2}\right)$. Assume that the inserts are followed by a series of queries without loss of generality. 
In this case, we would essentially do a sequential scan on the $o$ pages that may potentially be unsorted and further do an interpolation 
search on the sorted half of the buffer if required. We assume $o$ as the required threshold for sorting, i.e. at any point during a query, 
if the unsorted section of the buffer contains 
more than $o$ pages, we perform a sorting step before searching for the key using interpolation search, otherwise we simply do the sequential 
scan procedure. Note, every sorting step essentially demarcates sorted blocks of $o$ pages within the originally unsorted section of the buffer. For any point query 
that potentially falls into the orignial unsorted section, we perform interpolation search on these blocks, hence the number of 
pages sequentially scanned is reduced. Ideally, we want the cost of sorting and interpolation scan of these blocks to be less than the projected query cost of the unsorted section 
to be benefitial. 

\begin{equation}
	o\cdot log_2(o) + log_2(log_2(o)) < v + f_G \cdot Z_R \cdot f_p \cdot o 
\end{equation}

Assume $log_2(log_2(o)) \approx 1$ and $v=1$, we can simplify further: 
\begin{eqnarray}
	o\cdot log_2(o) + 1 < 1 + f_G \cdot Z_R \cdot f_p \cdot o \nonumber \\
	\Rightarrow o\cdot log_2(o) - f_G \cdot Z_R \cdot f_p \cdot o < 0 \nonumber \\
	\Rightarrow log_2(o) < f_G \cdot Z_R \cdot f_p  \nonumber \\
	\Rightarrow 0 < o < 2^{f_G \cdot Z_R \cdot f_p} 
	\label{eq:unsorted_pages_threshold}
\end{eqnarray}

\begin{eqnarray}
	f_p \cdot Z_R \cdot f_p^\prime \cdot \frac{S}{2} + 0.5\cdot \frac{S}{N_B} + 
	\left(1-\frac{S}{2\cdot N_B}\right) \cdot log_2\left(log_2\left(\frac{S}{2}\right)\right)+ \nonumber\\
	\left(1-\frac{S}{N_B}\right)\cdot log_B\left(N_B-S\right)) < (1+\delta) \cdot log_B\left(N_B\right) %\nonumber
	\label{eq:query_cost_buffer}
\end{eqnarray}

If we discard the $log_2\left(log_2\left(\frac{S}{2}\right)\right)$ as negligible and we
assume that $log_B\left(N_B\right) \approx log_B\left(N_B-S\right)$ because $S<<N_B$, then
we get the following.

\begin{eqnarray}
	f_p \cdot \frac{S}{2} + 0.5\cdot \frac{S}{N_B} + 
	\nonumber\\
	\left(1-\frac{S}{N_B}\right)\cdot log_B\left(N_B\right)) < (1+\delta) \cdot log_B\left(N_B\right) \Rightarrow\nonumber\\
	S\cdot \left(\frac{f_p}{2}+\frac{1}{2\cdot N_B}\right) < \left(\delta+\frac{S}{N_B}\right)\cdot log_B\left(N_B\right) \Rightarrow\nonumber\\
	S\cdot \left(\frac{f_p}{2}+\frac{1}{2\cdot N_B}\right) - \frac{S}{N_B}\cdot log_B\left(N_B\right) < \delta \cdot log_B\left(N_B\right) \Rightarrow\nonumber\\
	S\cdot \left(\frac{f_p}{2}+\frac{1}{2\cdot N_B} - \frac{log_B\left(N_B\right)}{N_B} \right)  < \delta \cdot log_B\left(N_B\right) \Rightarrow\nonumber\\
	S < \frac{2\cdot \delta \cdot N_B \cdot log_B\left(N_B\right)}{f_p\cdot N_B+1 - 2\cdot  log_B\left(N_B\right)}   \Rightarrow\nonumber\\
	p = \frac{S}{N_B} < \frac{2\cdot \delta \cdot log_B\left(N_B\right)}{f_p\cdot N_B+1 - 2\cdot  log_B\left(N_B\right)} 
	\label{eq:query_cost_buffer}
\end{eqnarray}

\Paragraph{Introducing parameterized sortedness}
We now try to introduce the concept of sortedness in the query cost, which will 
affect both cost of sequentially scanning the unsorted section as well as scanning the 
sorted section through the faster interpolation search. Let us assume we have a deterministic 
metric for sortedness quantified by $\alpha$. Then, the cost of a point query 
on \sysName{} from eq.~\eqref{eq:query_cost_buffer} can be modified as follows:

If we approximate $log_2\left(log_2\left(\frac{S}{2}\right)\right)\approx 1$ and we
assume that $log_B\left(N_B\right) \approx log_B\left(N_B-S\right)$ because $S<<N_B$, then
we get the following.

\begin{eqnarray}
	f_p \cdot Z_R \cdot f_p^\prime \cdot \frac{S}{2} + 0.5\cdot \frac{S}{N_B} + 
	\left(1-\frac{S}{2\cdot N_B}\right) \cdot 1+ \nonumber\\
	\left(1-\frac{S}{N_B}\right)\cdot log_B\left(N_B\right) < (1+\delta) \cdot log_B\left(N_B\right)\Rightarrow\nonumber\\
	f_p \cdot Z_R \cdot f_p^\prime \cdot \frac{S}{2} + 1+ 
	\left(1-\frac{S}{N_B}\right)\cdot log_B\left(N_B\right) < \nonumber\\ 
	(1+\delta) \cdot log_B\left(N_B\right)\Rightarrow\nonumber\\
	p=\frac{S}{N_B}<\frac{2\cdot \left(\delta\cdot log_B(N_B)-1\right)}{f_p \cdot Z_R \cdot f_p^\prime \cdot N_B - 2\cdot log_B(N_B)}
	\label{eq:query_cost_sortedness_metric}
\end{eqnarray}
